# Supplementary material for: Coordinate-independent model reductions of chemical reaction networks based on geometric singular perturbation theory
Source: arXiv:2508.03304 ancillary file (2026-01-19)
Supplement: Supplementary file 1 [file supplement1.pdf]

# Supplementary Materials: Part I

# List of all Singularly Perturbed Cases for the Reversible Michaelis-Menten Reaction Scheme and Further Information on the Normal Hyperbolicity Properties

# Coordinate-independent model reductions of chemical reaction networks based on geometric singular perturbation theory

Timothy Earl Figueroa Lapuz* Martin Wechselberger*

August 5, 2025

*School of Mathematics and Statistics, The University of Sydney, Camperdown NSW 2006, Australia

# 1 Complete list of singularly perturbed reversible Michaelis-Menten cases

In this section, we list all 67 singularly perturbed reversible Michaelis-Menten (MM) cases. We note that Tables 4, 5 and 6 in the main text lists the 23 singularly perturbed irreversible MM cases.

<table>
<tr><th>Subclass S.1</th><th>Subclass S.2a</th></tr>
<tr><td>i. $\beta, \delta = \mathcal{O}(\varepsilon), \alpha, \gamma = \mathcal{O}(1)$<br>ii. $\beta, \alpha, \delta = \mathcal{O}(\varepsilon), \gamma = \mathcal{O}(1)$<br>iii. $\beta, \gamma, \delta = \mathcal{O}(\varepsilon), \alpha = \mathcal{O}(1)$<br>Subclass S.2b<br>i. $\beta, \alpha, \delta = \mathcal{O}(\varepsilon), \gamma = \mathcal{O}\left(\frac{1}{\varepsilon}\right)$<br>ii. $\beta, \alpha, = \mathcal{O}(\varepsilon), \gamma = \mathcal{O}\left(\frac{1}{\varepsilon}\right), \delta = \mathcal{O}(1)$<br>iii. $\beta, \delta = \mathcal{O}(\varepsilon), \alpha = \mathcal{O}(1), \gamma = \mathcal{O}\left(\frac{1}{\varepsilon}\right)$<br>iv. $\beta = \mathcal{O}(\varepsilon), \alpha, \delta = \mathcal{O}(1), \gamma = \mathcal{O}\left(\frac{1}{\varepsilon}\right)$<br>v. $\beta, \gamma\delta = \mathcal{O}(\varepsilon), \alpha = \mathcal{O}\left(\frac{1}{\varepsilon}\right)$<br>vi. $\beta, \gamma = \mathcal{O}(\varepsilon), \alpha = \mathcal{O}\left(\frac{1}{\varepsilon}\right), \delta = \mathcal{O}(1)$<br>vii. $\beta, \delta = \mathcal{O}(\varepsilon), \alpha = \mathcal{O}\left(\frac{1}{\varepsilon}\right), \gamma = \mathcal{O}(1)$<br>viii. $\beta = \mathcal{O}(\varepsilon), \alpha = \mathcal{O}\left(\frac{1}{\varepsilon}\right), \gamma, \delta = \mathcal{O}(1)$<br>ix. $\beta, \delta = \mathcal{O}(\varepsilon), \alpha, \gamma = \mathcal{O}\left(\frac{1}{\varepsilon}\right)$<br>x. $\beta = \mathcal{O}(\varepsilon), \alpha, \gamma = \mathcal{O}\left(\frac{1}{\varepsilon}\right), \delta = \mathcal{O}(1)$<br>xi. $\beta = \mathcal{O}(1), \alpha, \delta = \mathcal{O}(\varepsilon), \gamma = \mathcal{O}\left(\frac{1}{\varepsilon}\right)$<br>xii. $\beta, \delta = \mathcal{O}(1), \alpha = \mathcal{O}(\varepsilon), \gamma = \mathcal{O}\left(\frac{1}{\varepsilon}\right)$<br>xiii. $\beta, \alpha = \mathcal{O}(1), \gamma = \mathcal{O}\left(\frac{1}{\varepsilon}\right), \delta = \mathcal{O}(\varepsilon)$<br>xiv. $\beta, \alpha, \delta = \mathcal{O}(1), \gamma = \mathcal{O}\left(\frac{1}{\varepsilon}\right)$</td><td>i. $\beta, \alpha, \gamma, \delta = \mathcal{O}(\varepsilon)$<br>ii. $\beta, \alpha, \gamma = \mathcal{O}(\varepsilon), \delta = \mathcal{O}(1)$<br>iii. $\beta, \alpha, \gamma = \mathcal{O}(\varepsilon), \delta = \mathcal{O}\left(\frac{1}{\varepsilon}\right)$<br>iv. $\beta, \alpha, = \mathcal{O}(\varepsilon), \gamma = \mathcal{O}(1), \delta = \mathcal{O}\left(\frac{1}{\varepsilon}\right)$<br>v. $\beta, \gamma = \mathcal{O}(\varepsilon), \alpha = \mathcal{O}(1), \delta = \mathcal{O}\left(\frac{1}{\varepsilon}\right)$<br>vi. $\beta = \mathcal{O}(\varepsilon), \alpha, \gamma = \mathcal{O}(1), \delta = \mathcal{O}\left(\frac{1}{\varepsilon}\right)$<br>Subclass S.3<br>i. $\beta = \mathcal{O}(1), \alpha = \mathcal{O}(\varepsilon), \gamma, \delta = \mathcal{O}\left(\frac{1}{\varepsilon}\right)$<br>ii. $\beta, \alpha, = \mathcal{O}(\varepsilon), \gamma, \delta = \mathcal{O}(1)$<br>Subclass S.4<br>i.$\beta, \alpha, = \mathcal{O}(\varepsilon), \gamma, \delta = \mathcal{O}\left(\frac{1}{\varepsilon}\right)$<br>ii. $\beta, \alpha, = \mathcal{O}(\varepsilon), \gamma, \delta = \mathcal{O}(1)$<br>iii. $\beta, \gamma = \mathcal{O}(\varepsilon), \alpha, \delta = \mathcal{O}(1)$<br>iv. $\beta = \mathcal{O}(\varepsilon), \alpha, \gamma, \delta = \mathcal{O}(1)$<br>v. $\beta = \mathcal{O}(\varepsilon), \alpha = \mathcal{O}(1), \delta, \gamma = \mathcal{O}\left(\frac{1}{\varepsilon}\right)$<br>vi. $\beta = \mathcal{O}(\varepsilon), \alpha, \delta = \mathcal{O}\left(\frac{1}{\varepsilon}\right), \gamma = \mathcal{O}(\varepsilon)$<br>vii. $\beta = \mathcal{O}(\varepsilon), \alpha, \delta = \mathcal{O}\left(\frac{1}{\varepsilon}\right), \gamma = \mathcal{O}(1)$<br>viii. $\beta = \mathcal{O}(\varepsilon), \alpha, \gamma, \delta = \mathcal{O}\left(\frac{1}{\varepsilon}\right)$</td></tr>
<tr><th>Subclass S.5a</th><th>Subclass 5b</th></tr>
<tr><td>i. $\beta = \mathcal{O}(1), \alpha, \gamma = \mathcal{O}(\varepsilon), \delta = \mathcal{O}\left(\frac{1}{\varepsilon}\right)$<br>ii. $\beta, \gamma = \mathcal{O}(1), \alpha = \mathcal{O}(\varepsilon), \delta = \mathcal{O}\left(\frac{1}{\varepsilon}\right)$<br>iii. $\beta, \alpha = \mathcal{O}(1), \gamma = \mathcal{O}(\varepsilon), \delta = \mathcal{O}\left(\frac{1}{\varepsilon}\right)$<br>iv. $\beta, \alpha, \gamma = \mathcal{O}(1), \delta = \mathcal{O}\left(\frac{1}{\varepsilon}\right)$</td><td>i. $\beta, \delta = \mathcal{O}\left(\frac{1}{\varepsilon}\right), \alpha, \gamma = \mathcal{O}(\varepsilon)$<br>ii. $\beta, \delta = \mathcal{O}\left(\frac{1}{\varepsilon}\right), \alpha = \mathcal{O}(\varepsilon), \gamma = \mathcal{O}(1)$<br>iii. $\beta, \gamma, \delta = \mathcal{O}\left(\frac{1}{\varepsilon}\right), \alpha = \mathcal{O}(\varepsilon)$<br>iv. $\beta, \delta = \mathcal{O}\left(\frac{1}{\varepsilon}\right), \alpha = \mathcal{O}(1), \gamma = \mathcal{O}(\varepsilon)$<br>v. $\beta, \delta = \mathcal{O}\left(\frac{1}{\varepsilon}\right), \alpha, \gamma = \mathcal{O}(1)$<br>vi. $\beta, \gamma, \delta = \mathcal{O}\left(\frac{1}{\varepsilon}\right), \alpha = \mathcal{O}(1)$</td></tr>
</table>

Table 1: The 43 Cases in Class S for the reversible MM.

| Subclass T.1 | Subclass T.2a |
|---|---|
| i. $\gamma, \delta = \mathcal{O}(\varepsilon), \alpha, \beta = \mathcal{O}(1)$ | i. $\gamma, \alpha, \delta = \mathcal{O}(\varepsilon), \beta = \mathcal{O}(1)$ |
| **Subclass T.2b** | **Subclass T.5c** |
| i. $\alpha = \mathcal{O}\left(\frac{1}{\varepsilon}\right), \beta = \mathcal{O}(1), \gamma, \delta = \mathcal{O}(\varepsilon)$<br>ii. $\alpha = \mathcal{O}\left(\frac{1}{\varepsilon}\right), \beta, \delta = \mathcal{O}(1), \gamma = \mathcal{O}(\varepsilon)$<br>iii. $\alpha = \mathcal{O}\left(\frac{1}{\varepsilon}\right), \beta, \gamma = \mathcal{O}(1), \delta = \mathcal{O}(\varepsilon)$<br>iv. $\alpha = \mathcal{O}\left(\frac{1}{\varepsilon}\right), \beta, \gamma, \delta = \mathcal{O}(1)$<br>v. $\alpha, \gamma = \mathcal{O}\left(\frac{1}{\varepsilon}\right), \beta = \mathcal{O}(1), \delta = \mathcal{O}(\varepsilon)$<br>vi. $\alpha, \gamma = \mathcal{O}\left(\frac{1}{\varepsilon}\right), \beta, \delta = \mathcal{O}(1)$<br>vii. $\alpha, \beta, \delta = \mathcal{O}\left(\frac{1}{\varepsilon}\right), \gamma = \mathcal{O}(\varepsilon)$<br>viii. $\alpha, \beta, \delta = \mathcal{O}\left(\frac{1}{\varepsilon}\right), \gamma = \mathcal{O}(1)$<br>ix. $\alpha, \delta, \gamma, \delta = \mathcal{O}\left(\frac{1}{\varepsilon}\right)$ | i. $\alpha, \gamma = \mathcal{O}(\varepsilon), \beta, \delta = \mathcal{O}(1)$<br>ii. $\alpha, \gamma = \mathcal{O}(\varepsilon), \beta = \mathcal{O}\left(\frac{1}{\varepsilon}\right), \delta = \mathcal{O}(1)$<br>iii. $\alpha = \mathcal{O}(\varepsilon), \beta = \mathcal{O}\left(\frac{1}{\varepsilon}\right), \gamma, \delta = \mathcal{O}(1)$ |

Table 2: The 14 cases in Class T for the reversible MM.

| Subclass R.1 | Subclass R.2a |
|---|---|
| i. $\beta = \mathcal{O}\left(\frac{1}{\varepsilon}\right), \alpha = \mathcal{O}(1), \gamma, \delta = \mathcal{O}(\varepsilon)$<br>ii. $\beta = \mathcal{O}\left(\frac{1}{\varepsilon}\right), \alpha, \gamma = \mathcal{O}(1), \delta = \mathcal{O}(\varepsilon)$ | i. $\beta = \mathcal{O}\left(\frac{1}{\varepsilon}\right), \alpha, \gamma, \delta = \mathcal{O}(\varepsilon)$<br>ii. $\beta = \mathcal{O}\left(\frac{1}{\varepsilon}\right), \alpha, \delta = \mathcal{O}(\varepsilon), \gamma = \mathcal{O}(1)$ |
| **Subclass R.2b** | |
| i. $\beta, \alpha = \mathcal{O}\left(\frac{1}{\varepsilon}\right), \gamma, \delta = \mathcal{O}(\varepsilon)$<br>ii. $\beta, \alpha = \mathcal{O}\left(\frac{1}{\varepsilon}\right), \gamma = \mathcal{O}(\varepsilon), \delta = \mathcal{O}(1)$<br>iii. $\beta, \alpha = \mathcal{O}\left(\frac{1}{\varepsilon}\right), \gamma = \mathcal{O}(1), \delta = \mathcal{O}(\varepsilon)$<br>iv. $\beta, \alpha = \mathcal{O}\left(\frac{1}{\varepsilon}\right), \gamma, \delta = \mathcal{O}(1)$<br>v. $\beta, \alpha, \gamma = \mathcal{O}\left(\frac{1}{\varepsilon}\right), \delta = \mathcal{O}(\varepsilon)$<br>vi. $\beta, \alpha, \gamma = \mathcal{O}\left(\frac{1}{\varepsilon}\right), \delta = \mathcal{O}(1)$ | |

Table 3: The 10 cases in Class R for the reversible MM.

## 1.1 Non-singularly perturbed cases

For completeness, we list here the non-singularly perturbed cases for both the irreversible and reversible MM.

| Non-cases | |
|---|---|
| i. $\alpha, \beta, \gamma = \mathcal{O}(1)$ | iii. $\alpha = \mathcal{O}(1), \beta, \gamma = \mathcal{O}\left(\frac{1}{\varepsilon}\right)$ |
| ii. $\alpha = \mathcal{O}(\varepsilon), \beta, \gamma = \mathcal{O}(1)$ | iv. $\alpha = \mathcal{O}(\varepsilon), \beta, \gamma = \mathcal{O}\left(\frac{1}{\varepsilon}\right)$ |

Table 4: The 4 cases that are not singularly perturbed for the irreversible MM.

| Non-cases | |
|---|---|
| i. $\alpha, \beta, \gamma, \delta = \mathcal{O}(1)$ | viii. $\alpha, \gamma, \delta = \mathcal{O}\left(\frac{1}{\varepsilon}\right), \beta = \mathcal{O}(1)$ |
| ii. $\alpha, \delta = \mathcal{O}(\varepsilon), \beta, \gamma = \mathcal{O}(1)$ | ix. $\alpha, \delta = \mathcal{O}(\varepsilon), \beta, \gamma = \mathcal{O}\left(\frac{1}{\varepsilon}\right)$ |
| iii. $\alpha = \mathcal{O}(\varepsilon), \beta, \gamma, \delta = \mathcal{O}(1)$ | x. $\alpha = \mathcal{O}(\varepsilon), \beta, \gamma = \mathcal{O}\left(\frac{1}{\varepsilon}\right), \delta = \mathcal{O}(1)$ |
| iv. $\alpha, \beta, \delta = \mathcal{O}(1), \gamma = \mathcal{O}(\varepsilon)$ | xi. $\alpha, \delta = \mathcal{O}(1), \beta = \mathcal{O}\left(\frac{1}{\varepsilon}\right), \gamma = \mathcal{O}(\varepsilon)$ |
| v. $\alpha, \beta, \gamma = \mathcal{O}(1), \delta = \mathcal{O}(\varepsilon)$ | xii. $\alpha, \gamma, \delta = \mathcal{O}(1), \beta = \mathcal{O}\left(\frac{1}{\varepsilon}\right)$ |
| vi. $\alpha, \delta = \mathcal{O}\left(\frac{1}{\varepsilon}\right), \beta = \mathcal{O}(1), \gamma = \mathcal{O}(\varepsilon)$ | xiii. $\alpha, = \mathcal{O}(1), \beta, \gamma = \mathcal{O}\left(\frac{1}{\varepsilon}\right), \delta = \mathcal{O}(\varepsilon)$ |
| vii. $\alpha, \delta = \mathcal{O}\left(\frac{1}{\varepsilon}\right), \beta, \gamma = \mathcal{O}(1)$ | xiv. $\alpha, \delta = \mathcal{O}(1), \beta, \gamma = \mathcal{O}\left(\frac{1}{\varepsilon}\right)$ |

Table 5: The 14 that are not singularly perturbed for the reversible MM.

## 2 Further information on normal hyperbolicity

This section is a supplement to Figure 5 in the main text. All statements assume $s, c \geq 0$ and the $\tilde{}$ notation above the parameter is suppressed.

We first note the following points for Figure 5 in the main text

- Some fast fibers shown are evolved in backward time to indicate which critical manifold is attracting, since the initial condition (IC) lies on a critical manifold.
- Some fast fibers shown has been shifted to the left of $\mathcal{W}^S((1,0)^b)$ to indicate which (subset of a) critical manifold is attracting, since the IC lies on a critical manifold.
- Some cases in Figure 5 in the main text shows only $\delta > 1$. Cases $\delta < 1$ and $\delta = 1$ are discussed below Table 7.

Table 6 and 7 now provide more information on the normal hyperbolicity of each case.

| Subclass (cases) | loss | attracting | repelling |
|---|---|---|---|
| S.1 (all) | - | all | - |
| S.2a (all) | $\{s = 0\}$ | $s > 0$ | - |
| S.2b (all) | - | all | - |
| R.1 (all) | - | all | - |
| R.2a (all) | $\{c = 1\}$ | $c < 1$ | $c > 1$ |
| R.2b (all) | all | - | - |
| T.1 (all) | - | all | - |
| T.2a (all) (a) $\{c = 1\}$, (b) $\{s = 0\}$ | $(s, c) = (0, 1)$ | (a) $s > 0$, (b) $c < 1$ | (a) -, (b) $c > 1$ |
| T.2b (all) | - | all | - |

Table 6: Summary of hyperbolicity properties for the irreversible cases. Refer to Tables 4, 5 and 6 in the main text for the parameter configurations.

| Subclass (cases) | loss | attracting | repelling |
|---|---|---|---|
| S.1 (all) | - | all | |
| S.2a (i) | $\{s = 0\}$ | $s > 0$ | - |
| S.2a (ii) | $\left\{s = s^d = \frac{\delta}{\delta-1}\right\}$ | $s < s^d$‡ | $s > s^d$‡ |
| S.2a (iii,iv,v,vi) | $\{s = s^d = 1\}$ | $s < s^d$ | $s > s^d$ |
| S.2b (all) | - | all | - |
| S.3 (all) | - | left branch | right branch |
| S.4 (ii) | $s^d = \frac{\gamma+\delta}{\delta-1}$† | $s < s^d$‡ | $s > s^d$‡ |
| S.4 (i,v) | $s^d = \frac{\gamma+\delta}{\delta}$† | $s < s^d$ | $s > s^d$ |
| S.4 (iii) | $s^d = \frac{\alpha+\delta}{\delta-1}$† | $s < s^d$‡ | $s > s^d$‡ |
| S.4 (iv) | $s^d = \frac{\alpha+\delta+\gamma}{\delta-1}$† | $s < s^d$‡ | $s > s^d$‡ |
| S.4 (vi,vii) | $s^d = \frac{\alpha+\delta}{\delta}$† | $s < s^d$ | $s > s^d$ |
| S.4 (viii) | $s^d = \frac{\alpha+\delta+\gamma}{\delta}$† | $s < s^d$ | $s > s^d$ |
| S.5a (a) $\{c = -\beta^{-1}s + \beta^{-1}\}$ (all) (b) $\{c = 1\}$ | $(s^d, c^d) = (1-\beta, 1)$ | (a) $s > s^d$ (b) $s < s^d$ | (a) $s < s^d$ (b) $s > s^d$ |
| S.5b (all) | - | $\{c = 0\}$ | $\{c = 1\}$ |
| R.1 (all) | - | all | - |
| R.2a (all) | $\{c = 1\}$ | $c < 1$ | $c > 1$ |
| R.2b (all) | all | - | - |
| T.1 (all) | - | all | - |
| T.2a (all) (a) $\{c = 1\}$, (b) $\{s = 0\}$ | $(s, c) = (0, 1)$ | (a) $s > 0$, (b) $c < 1$ | (a) -, (b) $c > 1$ |
| T.2b (all) | - | all | - |
| T.5c (i) | $(s^d, c^d) = \left(\frac{\delta(1-\beta)}{\delta-1}, 1\right)$ | $s < s^d$‡ | $s > s^d$‡ |
| T.5c (ii,iii) | - | - | all |

Table 7: Summary of hyperbolicity properties for the reversible cases. † = asymptote of the critical manifold. ‡ = only the $\delta - 1 > 0$ is shown. Refer to Section 1 for the parameter configurations.

The following points provide more details for Table 7.

- S.2a.ii: the location of the loss of normal hyperbolicity depends on $\delta$. The nontrivial eigenvalue for this case is $\delta(s-1) - s$.
  - Details of $\delta - 1 > 0$ are in Table 7.
  - If $\delta = 1$, then the vertical critical manifold $S_{0,1} = \{s = 0\}$ does not exist. The horizontal critical manifold $S_{0,2} = \{c = 1\}$ is attracting everywhere.
  - If $\delta < 1$, then the horizontal critical manifold $S_{0,2} = \{c = 1\}$ is attracting for $s > \frac{-\delta}{|\delta-1|}$.
- All of S.3: the nontrivial eigenvalue is given by $\delta(s - \beta - 1) - \gamma + 2\beta\delta c$.
  - Setting the nontrivial eigenvalue to zero gives $c = \frac{\delta(1+\beta-s)+\gamma}{2\beta\delta}$ and the two critical manifolds are on the left and right of this line.
  - The $s$-intercept of the left critical manifold is at $(1, 0)$ and so we can conclude that the left branch is the attracting branch.
- Cases S.4.ii,iii,iv: critical manifolds have $g(s) = s - \delta s$ and a horizontal asymptote $c = 1$; see Definition 5 in the main text. The nontrivial eigenvalue is given by $\delta s - s - \delta - \Delta$, where $\Delta = \{\alpha, \gamma, \alpha + \gamma\}$.

- Details of $\delta - 1 > 0$ are in Table 7. The left branch $s < s^d$ is attracting.
  - As $s \to -\infty$, we have $c \to 1^-$. Hence, the left branch is below the horizontal asymptote. This is because the critical manifold is a hyperbola and so it does not cross its asymptotes.
  - We have that $s_{int} > 1$.
- If $\delta - 1 < 1$, then the right branch is attracting. The vertical asymptote $s = s^d$ is at a negative value.
  - As $s \to +\infty$, we have $c \to 1^-$. Hence, the right branch is below the horizontal asymptote. This is because the critical manifold is a hyperbola and so it does not cross its asymptotes.
- If $\delta = 1$, then the two critical manifolds merge to give a single critical manifold $\left\{c = \frac{1}{1+\Delta}\right\}$ where $\Delta = \{\alpha, \gamma, \alpha + \gamma\}$. It is attracting everywhere.

- Case T.5c.i: the nontrivial eigenvalue is $\delta(\beta - 1) + \delta s - s$.
  - Details for $\delta > 1$ is in Table 7.
  - If $\delta < 1$, then the critical manifold is attracting for $s > \frac{\delta(1-\beta)}{-|\delta-1|}$.
  - If $\delta = 1$, then the nontrivial eigenvalue is $\beta - 1$, so its normal hyperbolicity now depends on $\beta$.

**Remark 1.** *Case T.5c.i, with $\beta, \delta = \mathcal{O}(1), \alpha, \gamma = \mathcal{O}(\varepsilon)$ is the only case where the loss of normal hyperbolicity at a point is due to the tangency of $N_0$ with the critical manifold. The rest of the degeneracies that occur at a point are due to intersections of critical manifolds. In fact, $s^d = \frac{\delta(1-\beta)}{\delta-1}$ is a contact point of order 1 away from $\beta = 1$; see [2, 1] for details.*

# References

[1] I. Lizarraga, R. Marangell, and M. Wechselberger, *Slow Unfoldings of Vontact Singularities in Singularly Perturbed Systems Beyond the Standard Form*, J. Nonlinear Sci., 30 (2020), pp. 3161–3198.

[2] M. Wechselberger, *Geometric singular perturbation theory beyond the standard form*, vol. 6 of Frontiers in Applied Dynamical Systems: Reviews and Tutorials, Springer, 2020.
