# Supplementary material for: Coordinate-independent model reductions of chemical reaction networks based on geometric singular perturbation theory
Source: arXiv:2508.03304 ancillary file (2026-01-19)
Supplement: Supplementary file 2 [file supplement2.pdf]

# Supplementary Materials: Part II

# Selected Sample Model Reductions of the Michaelis-Menten Reaction Scheme and Discussion of Leading-Order Agreement with QSSA for the Irreversible Case

# Coordinate-independent model reductions of chemical reaction networks based on geometric singular perturbation theory

Timothy Earl Figueroa Lapuz* Martin Wechselberger*

August 5, 2025

## 1 Selected model reductions

**The classical standard quasi-steady-state approximation (sQSSA): $\varepsilon := \beta$, $\alpha, \gamma = \mathcal{O}(1)$ and $\delta = 0$ (Case S.1.i)** In [1], a QSSA for $c$ is applied. Decades later, [4] appeals to singular perturbation theory to justify the sQSSA for the case $\varepsilon_{HTA} := \beta \ll 1$[1]. Here, we use our coordinate-independent geometric singular perturbation theory (ci-GSPT) tools to calculate the model reduction.

For this parameter configuration, we have

$$\begin{aligned}\begin{pmatrix}\frac{ds}{dt}\\ \frac{dc}{dt}\end{pmatrix} &= \begin{pmatrix}0\\1\end{pmatrix}(s(1-c)-\alpha c-\gamma c)+\varepsilon\left(\begin{pmatrix}-s(1-c)\\0\end{pmatrix}+\alpha\begin{pmatrix}c\\0\end{pmatrix}\right)\\ &= N_0 f_0(s,c)+\varepsilon F_1(s,c).\end{aligned}$$

The set $S_0 = \{(s,c)\,|\,F_0(s,c) = 0\}$ is a one-dimensional manifold and is as a graph over $s$ is as follows

$$c_0(s) = \frac{s}{\alpha+\gamma+s}$$

and hence an embedding $\phi(s)$ of slow manifold $S_0^{\varepsilon}$ is

$$\phi(s,\varepsilon) = \phi_0(s) + \ldots = \begin{pmatrix}s\\ \frac{s}{\alpha+\gamma+s}\end{pmatrix} + \cdots.$$

*School of Mathematics and Statistics, The University of Sydney, Camperdown NSW 2006, Australia

[1] According to [6], [10] considers the $e_0 \ll s_0$ (as well as the case $e_0 = s_0$) before [4] and "anticipates some aspects of their scaling arguments". See [6] for the historical context of [4].

This critical manifold is of Form 1 and so this case is in Subclass S.1. The nontrivial eigenvalue is given by

$$Df_0N_0\big|_{S_0} = \begin{pmatrix}1-c & -\alpha-\gamma-s\end{pmatrix}\begin{pmatrix}0\\1\end{pmatrix}\Bigg|_{S_0} = -(\alpha+\gamma+s).$$

We then have the following left inverse and projection operator

$$D\phi_0^L\Pi_0^S = \begin{pmatrix}1 & 0\end{pmatrix}\begin{pmatrix}1 & 0\\ \frac{\alpha+\gamma}{(\alpha+\gamma+s)^2} & 0\end{pmatrix},$$

which we apply on the $F_1$ term. The reduced vector field on $S_0$ is given as

$$\frac{ds}{dt} = -\varepsilon R_1(s) = -\varepsilon\frac{\gamma s}{\alpha+\gamma+s}$$

and the leading-order product formation rate may be calculated as

$$\frac{dp}{dt} = \varepsilon R_1(s) = \varepsilon\frac{\gamma s}{\alpha+\gamma+s}. \tag{1.1}$$

**The classical reverse QSSA (rQSSA): $\varepsilon := \beta^{-1}$, $\alpha,\gamma = \mathcal{O}(1)$ and $\delta = 0$ (Case R.1.i)** In [8], it is mentioned in passing that when $\beta$ is large, then the rQSSA is the "appropriate assumption".

For this parameter configuration, we have

$$\begin{pmatrix}\frac{ds}{dt}\\ \frac{dc}{dt}\end{pmatrix} = \frac{1}{\varepsilon}N_0f_0(s,c) + F_1(s,c) = \frac{1}{\varepsilon}\begin{pmatrix}1\\0\end{pmatrix}(\alpha c - s(1-c)) + \begin{pmatrix}0\\ s(1-c)-\alpha c-\gamma c\end{pmatrix}.$$

A rescaling of time $\tau = t/\varepsilon$ gives

$$\begin{pmatrix}\frac{ds}{d\tau}\\ \frac{dc}{d\tau}\end{pmatrix} = N_0f_0(s,c) + \varepsilon F_1(s,c). \tag{1.2}$$

The set $S_0 = \{(s,c)\,|\,F_0(s,c)=0\}$ is a one-dimensional manifold and is as a graph over $s$ is as follows

$$c_0(s) = \frac{s}{\alpha+s}$$

and hence we can write an embedding $\phi(s)$ of the slow manifold $S_0^\varepsilon$ as follows

$$\phi(s,\varepsilon) = \phi_0 + \cdots = \begin{pmatrix}s\\ \frac{s}{\alpha+s}\end{pmatrix} + \cdots.$$

The critical manifold is of Form 1 and so this is a case in Subclass R.1. The nontrivial eigenvalue is given by

$$Df_0N_0\big|_{S_0} = \begin{pmatrix}-(1-c) & \alpha+s\end{pmatrix}\begin{pmatrix}1\\0\end{pmatrix}\Bigg|_{S_0} = \frac{s}{\alpha+s} - 1.$$

We then have the following left inverse and projection operator

$$D\phi_0^L \Pi_0^S = \begin{pmatrix} 1 & 0 \end{pmatrix} \begin{pmatrix} 0 & \frac{(\alpha+s)^2}{\alpha} \\ 0 & 1 \end{pmatrix}.$$

Applying this to $F_1$, we obtain the reduded vector field on $S_0$, given as

$$\frac{ds}{d\tau} = -\varepsilon R_1(s) = -\varepsilon \frac{\gamma s(\alpha+s)}{\alpha}. \tag{1.3}$$

From the conserved quantity $s + \beta c + p = 1$, we then have that (noting the time scale $\tau$)

$$\frac{ds}{d\tau}\left(1 + \frac{1}{\varepsilon} c_0'(s)\right)\frac{ds}{dt} + \frac{dp}{d\tau} = 0.$$

We then obtain that the approximate product formation is

$$\frac{dp}{d\tau} = c_0'(s) R_1(s) = \frac{\gamma s}{s+\alpha}. \tag{1.4}$$

**Remark 1.** *Recall that Case R.1.i undergoes a rapid equilibriation due to the IC at* $(1,0)$. *The substrate depletion rate* (1.3) *applies when we change the IC.*

**A reversible sQSSA case: $\varepsilon := \beta$, $\alpha, \gamma, \delta = \mathcal{O}(1)$ (Case S.4.iv)** For this parameter configuration, we have

$$\begin{aligned}\begin{pmatrix} \frac{ds}{dt} \\ \frac{dc}{dt} \end{pmatrix} &= \begin{pmatrix} 0 \\ 1 \end{pmatrix}(s(1-c) - (\alpha+\gamma)c + \delta(1-s)(1-c)). + \varepsilon \begin{pmatrix} -s(1-c) + \alpha c \\ -c(1-c) \end{pmatrix} \\ &= N_0 f_0(s,c) + \varepsilon F_1(s,c).\end{aligned}$$

The set $S_0 = \{(s,c) \,|\, F_0(s,c) = 0\}$ is a one-dimensional manifold and is a graph over $s$ is as follows

$$c_0(s) = \frac{\delta + s - \delta s}{\alpha + \gamma + \delta + s - \delta s} \tag{1.5}$$

and hence an embedding $\phi(s)$ of $S_0^\varepsilon$ is as follows

$$\phi(s,\varepsilon) = \phi_0(s) + \ldots = \begin{pmatrix} s \\ \frac{\delta+s-\delta s}{\alpha+\gamma+\delta+s-\delta s} \end{pmatrix} + \ldots.$$

This is a critical manifold of Form 4 and so this case is in Subclass S.4. The nontrivial eigenvalue is then given by

$$\begin{aligned} Df_0 N_0\big|_{S_0} &= \begin{pmatrix} (1-\delta)(1-c) & \delta(s-1) - (\alpha+\gamma+s) \end{pmatrix} \begin{pmatrix} 0 \\ 1 \end{pmatrix}\Bigg|_{S_0} \\ &= \delta(s-1) - (\alpha+\gamma+s). \end{aligned}$$

We then have the following left inverse and projection operator

$$D\phi_0^L \Pi_0^S = \begin{pmatrix} 1 & 0 \end{pmatrix} \begin{pmatrix} 1 & 0 \\ \frac{(\alpha+\gamma)(1-\delta)}{(\alpha+\gamma+\delta+s-\delta s)^2} & 0 \end{pmatrix}.$$

Applying this to $F_1$, we obtain the reduced vector field on $S_0$, given as

$$\frac{ds}{dt} = -\varepsilon R_1(s) = -\varepsilon \frac{\gamma s - \alpha\delta + \alpha\delta s}{\alpha + \gamma + \delta + s - \delta s} \tag{1.6}$$

and the leading-order approximate product formation rate may be calculated as

$$\frac{dp}{dt} = \varepsilon R_1(s) = \varepsilon \frac{\gamma s - \alpha\delta + \alpha\delta s}{\alpha + \gamma + \delta + s - \delta s}. \tag{1.7}$$

**Remark 2.** *The nondimensional system* (1.6) *matches the dimensional reduced equation stated in equation (15) of [5] and equation (4) in [3]. Furthermore, in [5, 3], they looked at the limit $e_0 \to 0$ in the dimensional equations, which gives the dimensional critical manifold $\{C = 0\}$. Now, we have used $e_0$ as the reference scale i.e. $C = e_0 c$ and so $e_0 \to 0$ means that we are 'zooming in' to the dimensional critical manifold given by $\{C = 0\}$. If we convert the dimensional critical manifold given by $C = \mathcal{O}(e_0)$ in [3] (the approximation after equation (4)), then it matches our dimensionless critical manifold in* (1.5).

## 2 Leading-order agreement with QSSAs

One may find that the
model reductions in the main text may not match the QSSAs of literature, particularly for the irreversible MM. However, [3] extensively discuss the agreement to leading-order in the small parameter between reductions via Tikhonov-Fenichel (i.e. using the ci-GSPT tools) and QSSA.

In this section, we discuss the 'apparent' discrepancies for the leading-order product formation rate of the irreversible MM reaction scheme $\delta = 0$. The product formation rate is given bythe last equation of system (2.5) in the main text, as follows

$$\frac{dp}{dt} = \beta\gamma c(s, \varepsilon) \tag{2.1}$$

where $c(s, \varepsilon) = c_0(s) + \varepsilon c_1(s) + \cdots$ and typically we take the leading-order approximation $c_0(s)$ for the critical manifold $S_0$. From there, we can obtain a dimensional version given by

$$\frac{dP}{dT} = k_2 C(S), \tag{2.2}$$

where $C(S) = e_0 c_0(s)$. This is also in the last equation of (2.4) in the main text.

However, we do note that this leading-order approximation of product formation rates apply only to normally hypeborbolic critical manifolds that can be written as a graph over $s$, so that we can make the approximation $c(s, \varepsilon) \approx c_0(s)$ (see Section 3.2 of the main text).

We now discuss the relationship between (2.2) and the product formation rates derived literature. The validity conditions referred to are defined in Table 7 of the main text.

### Class S

**Subclass S.1** The dimensional product formation rates for this subclass is of the form

$$\frac{dP}{dT} = k_2 e_0 \frac{S}{S + \Delta} \tag{2.3}$$

where $\Delta = \{K, K_R, K_M\}$ and $K_M = K + K_R = \frac{k_2 + k_{-1}}{k_1}$. We then have the following:

- For Case S.1.i, we have that $\varepsilon := \beta, \alpha = \frac{k_{-1}}{k_1 s_0}, \gamma = \frac{k_2}{k_1 s_0} = \mathcal{O}(1)$. With these assumptions, $K_R$ is of the same order as $K$ and so $\Delta = K_M$ and matches (2.4). The dimensionless version is given by equation (1.1).
- For Case S.1.ii, we have that $\varepsilon := \beta, \alpha = \mathcal{O}(\varepsilon), \gamma = \mathcal{O}(1)$. With these assumptions, $K_R$ is relatively smaller than $K$ and so $\Delta = K$.
- For Case S.1.iii $\varepsilon := \beta, \gamma = \frac{k_2}{k_1 s_0} = \mathcal{O}(\varepsilon), \alpha = \mathcal{O}(1)$. With these assumptions, $K$ is relatively smaller than $K_R$ and so $\Delta = K_R$.

**Subclass S.2a** The one case in this subclass is Case S.2a.i, where $\varepsilon := \beta, \alpha, \gamma = \mathcal{O}(\varepsilon)$. We note that this case has two critical manifolds $S_{0,1} \cup S_{0,2} = \{s = 0\} \cup \{c = 1\}$. The critical manifold $S_{0,2}$ for $s > 0$ is normally hyperbolic and attracting.

With the given parameter assumptions and noting that $s > 0$, the dimensional parameter $K_M$ may be taken to be relatively small compared to $S$ in equation (2.3). This then gives the dimensional product formation rate

$$\frac{dP}{dT} = k_2 e_0.$$

**Subclass S.2b** All cases in this subclass have $\alpha = \mathcal{O}\left(\frac{1}{\varepsilon}\right)$ and/or $\gamma = \mathcal{O}\left(\frac{1}{\varepsilon}\right)$. Therefore, the modification to equation (2.3) is

$$\frac{dP}{dT} = k_2 e_0 \frac{S}{\Delta\left(1 + \frac{S}{\Delta}\right)} \approx k_2 e_0 \frac{S}{\Delta}$$

where $\Delta = \{K_M, K, K_R\}$, depending on whether $\alpha$ and/or $\gamma$ is relatively large.

**Literature product formation rate** For the sQSSA, the dimensional product formation rate usually stated in literature is

$$\frac{dP}{dT} = k_2 e_0 \frac{S}{K_M + S} \tag{2.4}$$

for the condition $\varepsilon_{HTA} \ll 1$ (see e.g. substrate depletion in [4]) and $\varepsilon_{SS} \ll 1$[2] (e.g. see [8] and the $C(S)$ function after applying sQSSA in [9]). The product formation rate derived from critical manifolds are therefore approximations of equation (2.4).

[2]See Table 7 of the main text for the definition of $\varepsilon_{SS}$.

### Class T

[8] derive the dimensional product formation rate

$$\frac{dP}{dT} = k_2 e_0 \frac{S}{S + K_M}. \tag{2.5}$$

for condition $\varepsilon_{BdBS} \ll 1$[3] by making asymptotic expansions. This is the same as (2.4) for the sQSSA.

The dimensional product formation rate for Case T.1.i, where $\varepsilon := \gamma, \alpha, \beta = \mathcal{O}(1)$, is given by is

$$\frac{dP}{dT} = k_2 e_0 \frac{S}{S + K_R}.$$

Since $\gamma$ is small, it is only $K_R$ that appears in the denominator (see also equation (3.18) in the main text for the nondimensional version). In fact, the same modifications apply depending on the relative sizes of $\alpha$ and $\gamma$ as in our previous discussion for Class S.

Now, a coordinate transformation is typically the first step for a tQSSA and so the dimensional product formation rate in the $(\bar{S}, C)$-space is

$$\frac{dP}{dT} = k_2 \left( \frac{1}{2}(e_0 + K_M + \bar{S}) - \frac{1}{2}\sqrt{(e_0 + K_M + \bar{S})^2 - 4e_0\bar{S}} \right), \tag{2.6}$$

where $\bar{S} = S + C$ (see e.g. [2] and the $C(\bar{S})$ function after applying tQSSA in [11]). Substituting $\bar{S} = S + C$ and $C(S) = e_0 \frac{S}{k_M + S}$ in (2.6) results in (2.5).

### Class R

[7] derive the dimensional product formation rate

$$\frac{dP}{dT} = k_2 \frac{e_0 S}{K_R + S}. \tag{2.7}$$

for the rQSSA for the condition $\varepsilon_{HTA}^{-1} \ll 1$ and $\varepsilon_{SM,SS} \ll 1$[4].

The dimensional product formation rate for Case R.1.i, where $\varepsilon := \beta^{-1}, \alpha, \gamma = \mathcal{O}(1)$, is given by

$$\frac{dP}{dT} = k_2 \frac{e_0 S}{K_R + S} \tag{2.8}$$

which matches (2.7). We note that the dimensionless version is given by equation (1.4).

Depending on the relative size of $\alpha$, the same modifications as in Class S applies here. However, we do note that:

- Cases in Subclass R.2a have two critical manifolds $S_{0,1} \cup S_{0,2} = \{s = 0\} \cup \{c = 1\}$. The critical manifold $S_{0,1}$ for $0 \le c < 1$ is attracting, but cannot be written as a graph over $s$.
- Cases in Subclass R.2b have a single critical manifold that is degenerate everywhere and so we cannot apply the approximation $c(s, \varepsilon) \approx c_0(s)$.

[3] See Table 7 of the main text for the definition of $\varepsilon_{BdBS}$.

[4] See Table 7 of the main text for the definition of $\varepsilon_{SM,SS}$.

**Resolving an apparent discrepancy** Segel and Slemrod [9] found the following product formation rate

$$\frac{dP}{dT} = k_2 \frac{e_0 S}{K_R}, \tag{2.9}$$

for a case where $\varepsilon_{SS}^{-1} \ll 1$ i.e. $s_0 + K_M \ll e_0$. Only cases in Subclass R.1 and R.2a satisfies $\varepsilon_{SS}^{-1} \ll 1$ (see Table 7 of the main text). The apparent discrepancy is that the relevant critical manifolds of Subclass R.1 and R.2a does not appear to give the desired linear product formation rate (2.9). Furthermore, cases in these subclasses undergo a rapid equilibriation and so there should not be any product formation due to the trivial reduction.

Figure 5 in [9] is an example of a case where $\varepsilon_{SS}^{-1} \ll 1$. Translating the parameters values they chose for this example, we have

$$\varepsilon_{SS} = \frac{\beta}{1 + \alpha + \gamma} = 50, \quad \sigma = \frac{1}{\alpha + \gamma} = 1, \quad \kappa = \frac{\alpha}{\gamma} = 1,$$

we obtain $\alpha = 0.5, \gamma = 0.5$ and $\beta = 100$, which is Case R.1.i (equation (1.4) shows it nondimensional product formation rate) and indeed satisfies $\varepsilon_{SS}^{-1} \ll 1$. Segel and Slemrod then calculate the 'knee' coordinates. It is approximately $(s_k, c_k) = (0.005, 0.02)$, which is approximately the coordinates of the IC of the reduced flow on the critical manifold.

Once it is known that the values of the knee coordinates are small, we can conclude that $s_k \ll s_0 \implies s_k \ll K_M \implies s_k \ll K_R$, since Segel and Slemrod also restricted to 'interesting cases' where $k_{-1} \approx k_2$. With this, (2.8) then simplifies to the desired linear product formation rate (2.9).

Hence, after the transient, the flow is near the origin and follows a linear product formation rate. This is coherent with a rapid equilibriation, where the layer flow rapidly approaches the origin in the singular limit and and resolves the apparent discrepancy.

# References


[1] G. E. Briggs and J. B. S. Haldane, *A note on the kinetics of enzyme action*, Biochem. J., 19 (1925), pp. 338–339.

[2] J. Eilertsen and S. Schnell, *The quasi-steady-state approximations revisited: Timescales, small parameters, singularities, and normal forms in enzyme kinetics*, Math. Biosci., 325 (2020), p. 108339.

[3] A. Goeke, S. Walcher, and E. Zerz, *Classical quasi-steady state reduction—a mathematical characterization*, Phys. D, 345 (2017), pp. 11–26.

[4] F. G. Heineken, H. M. Tsuchiya, and R. Aris, *On the mathematical status of the pseudo-steady state hypothesis of biochemical kinetics*, Math. Biosci., 1 (1967), pp. 95–113.

[5] L. Noethen and S. Walcher, *Tikhonov's theorem and quasi-steady state*, Discrete Contin. Dyn. Syst. Ser. B, 16 (2011), pp. 945–961.

[6] M. R. Roussel, *Heineken, Tsuchiya and Aris on the mathematical status of the pseudo-steady state hypothesis: A classic from volume 1 of Mathematical Biosciences*, Math. Biosci., 318 (2019), p. 108274.

[7] S. Schnell and P. K. Maini, *Enzyme kinetics at high enzyme concentration*, Bull. Math. Bio., 62 (2000), pp. 483–499.

[8] ——, *Enzyme kinetics far from the standard quasi-steady-state and equilibrium approximations*, Math. Comput. Model., 35 (2002), pp. 137–144.

[9] L. A. Segel and M. Slemrod, *The quasi-steady-state assumption: a case study in perturbation*, SIAM Rev., 31 (1989), pp. 446–477.

[10] P. A. T. Swoboda, *The kinetics of enzyme action*, Biochim. Biophys. Acta, 23 (1957), pp. 70–80.

[11] A. R. Tzafriri, *Michaelis-Menten Kinetics at High Enzyme Concentrations*, Bull. Math. Biol., 65 (2003), pp. 1111–1129.
