# Supplementary material for: Coordinate-independent model reductions of chemical reaction networks based on geometric singular perturbation theory
Source: arXiv:2508.03304 ancillary file (2026-01-19)
Supplement: Supplementary file 3 [file supplement3.pdf]

# Supplementary Materials: Part III

# Equilibrium Analysis of the Michaelis-Menten Reaction Scheme

# Coordinate-independent model reductions of chemical reaction networks based on geometric singular perturbation theory

Timothy Earl Figueroa Lapuz* Martin Wechselberger*

August 5, 2025

## 1 Proofs for the stability of the relevant equilibrium in the Michaelis-Menten reaction scheme

The 2D system arising from the reversible Michaelis-Menten (MM) (2.8) in the main text has two equilibra at

$$s^*_\pm = -\frac{\alpha}{2} - \frac{\alpha(\delta(\beta-1) \pm \sqrt{\Delta})}{2\gamma + 2\alpha\delta}, \quad c^*_\pm = \frac{\gamma + \delta(\alpha+\beta+1) \pm \sqrt{\Delta}}{2\beta\delta} \tag{1.1}$$

where $\Delta = (\gamma + \delta(\alpha+\beta+1))^2 - 4\beta\delta^2$. The Jacobian of the 2D system (2.7) in the main text, not evaluated at a point, is also as follows

$$J_{rev} = \begin{pmatrix} \beta(c-1) & \beta(\alpha+s) \\ \delta(c-1) - c + 1 & \delta(s+\beta c - 1) - (\alpha+\gamma+s) + \beta\delta(c-1) \end{pmatrix}. \tag{1.2}$$

The eigenvalues from the Jacobian are given by

$$\lambda_{1,2} = \frac{1}{2}(trJ_{rev} \pm \sqrt{(trJ_{rev})^2 - 4detJ_{rev}}). \tag{1.3}$$

**Proposition 1.** *The equilibria $(s^*_-, c^*_-)$ and $(s^*_+, c^*_+)$ exists for $\alpha, \beta, \gamma, \delta > 0$.*

*Proof.* For $\alpha, \beta, \gamma, \delta > 0$, we have that

$$\begin{aligned} &(\gamma + \delta(\alpha+\beta+1))^2 - 4\beta\delta^2 \\ &= \left(\gamma + \delta(\alpha+\beta+1) + 2\sqrt{\beta}\delta\right)\left(\gamma + \delta(\alpha+\beta+1) - 2\sqrt{\beta}\delta\right) \\ &= \left(\gamma + \delta(\alpha+\beta+1) + 2\sqrt{\beta}\delta\right)\left(\gamma + \alpha\delta + \delta(\sqrt{\beta}-1)^2\right) \\ &\geq 0. \end{aligned}$$

This means $\Delta \geq 0$ in (1.1) and hence the equilibria are real. ☐

*School of Mathematics and Statistics, The University of Sydney, Camperdown NSW 2006, Australia

Note that the formula for the equilibria in (1.1) is undefined at $\delta = 0$. However, we note that $(s_-^*, c_-^*) \to (0,0)$ as $\delta \to 0$. In fact, we can calculate that there is a unique equilibrium at the origin for the 2D system arising from the irreversible MM.

**Lemma 1.** *For $\alpha, \beta, \gamma > 0$ and $\delta \geq 0$, $0 \leq c_-^* < 1$.*

*Proof.* For the upper bound of $c_-^*$, we need to prove that

$$\begin{aligned} c_-^* &< 1 \\ \gamma + \delta(\alpha+\beta+1) - \sqrt{\Delta} &< 2\beta\delta \\ \gamma + \delta(\alpha+\beta+1) - 2\beta\delta &< \sqrt{\Delta}. \end{aligned}$$

Now, consider

$$\begin{aligned} \gamma + \alpha\delta &> 0 \\ -\delta(\beta+1) + \delta(\beta+1) + \gamma + \alpha\delta &> 0 \\ -\delta(\beta+1) &> -\gamma - \delta(\alpha+\beta+1) \\ -4\beta\delta^2(\beta+1) &> -4\beta\delta\left(\gamma + \delta(\alpha+\beta+1)\right) \\ -4\beta\delta^2 &> -4\beta\delta\left(\gamma + \delta(\alpha+\beta+1)\right) + 4\beta^2\delta^2 \\ (\gamma + \delta(\alpha+\beta+1))^2 - 4\beta\delta^2 &> (\gamma + \delta(\alpha+\beta+1))^2 \\ &\quad - 4\beta\delta\left(\gamma + \delta(\alpha+\beta+1)\right) + 4\beta^2\delta^2 \\ \Delta &> \left(\gamma + \delta(\alpha+\beta+1) - 2\beta\delta\right)^2. \end{aligned} \tag{1.4}$$

Taking the square root of both sides yields the desired result. For the lower bound of $c_-^*$, consider

$$\begin{aligned} 4\beta\delta^2 &\geq 0 \\ 0 &\geq -4\beta\delta^2 \\ (\gamma + \delta(\alpha+\beta+1))^2 &\geq \Delta \, (\geq 0) \\ \gamma + \delta(\alpha+\beta+1) - \sqrt{\Delta} &\geq 0 \\ c_-^* &\geq 0. \end{aligned} \tag{1.5}$$

Hence, we have shown that $0 \leq c_-^* < 1$. □

**Lemma 2.** *For $\alpha, \beta, \gamma > 0$ and $\delta \geq 0$, $c_+^* > 1$.*

*Proof.* To show the lower bound, we need to show

$$\begin{aligned} c_+^* &> 1 \\ \gamma + \delta(\alpha+\beta+1) + \sqrt{\Delta} &> 2\beta\delta \\ \sqrt{\Delta} &> 2\beta\delta - \gamma - \delta(\alpha+\beta+1). \end{aligned}$$

Following similar steps in (1.4) leads to the desired result. □

**Lemma 3.** *For $\alpha, \beta, \gamma > 0$ and $\delta \geq 0$, $s_-^* \geq 0$ and $s_+^* < 0$. .*

*Proof.* Setting the first ODE in system (2.8) of the main paper to zero gives $s = \frac{\alpha c}{1-c}$, giving the desired result. □

Lemma 3 shows that $(s_-^*, c_-^*)$ is the biologically relevant equilibrium. The following gives an upper bound to $s_-^*$.

**Lemma 4.** *For $\alpha, \beta, \gamma > 0$ and $\delta \geq 0$, $s_-^* < 1$.*

*Proof.*

$$\begin{aligned}
4(\gamma + \alpha\delta)(\gamma + \alpha\gamma + \alpha\beta\delta) &> 0 \\
\alpha^2\left((\gamma + \delta(\alpha + \beta + 1))^2 - 4\beta\delta^2\right) + & \\
4(\gamma + \alpha\delta)(\gamma + \alpha\gamma + \alpha\beta\delta) &> \alpha^2\left((\gamma + \delta(\alpha + \beta + 1))^2 - 4\beta\delta^2\right) \\
\left(2(\gamma + \alpha\delta) + \alpha(\gamma + \alpha\delta) + \alpha\delta(\beta - 1)\right)^2 &> \alpha^2\left((\gamma + \delta(\alpha + \beta + 1))^2 - 4\beta\delta^2\right) \\
2(\gamma + \alpha\delta) + \alpha(\gamma + \alpha\delta) + \alpha\delta(\beta - 1) &> \alpha\sqrt{(\gamma + \delta(\alpha + \beta + 1))^2 - 4\beta\delta^2} \\
1 &> s_-^*.
\end{aligned}$$

□

**Lemma 5.** *For $\alpha, \beta, \gamma > 0$ and $\delta \geq 0$, we have the following statements about $J_{rev}$ in (1.2).*

1. *$trJ_{rev} < 0$.*
2. *$detJ_{rev} \geq 0$.*
3. *$(trJ_{rev})^2 - 4detJ_{rev} > 0$.*

*Proof.* 1. $trJ_{rev} < 0$. The trace is given by

$$\beta(c - 1) + \delta(s + \beta c - 1) - (\alpha + \gamma + s)\beta\delta(c - 1).$$

Observe each term is nonnegative from the conserved quantities (2.7) in the main text. In fact, we have that $c_-^* - 1 > 0$ from Lemma 1. Hence, the trace for the equilibrium is strictly negative.

2. $detJ_{rev} \geq 0$.

$$\begin{aligned}
detJ_{rev} &= \beta(c - 1)\Big(\delta(s + \beta c - 1) - (\alpha + \gamma + s) + \beta\delta(c - 1)\Big) \\
&\quad - \beta(\alpha + s)(\delta - 1)(c - 1) \\
&= \beta(c - 1)\Big(\delta(s + \beta c - 1) - (\alpha + \gamma + s) + \beta\delta(c - 1) - (\alpha + s)(\delta - 1)\Big) \\
&= \beta(c - 1)\Big(\delta(s + \beta c - 1) - \gamma + \beta\delta(c - 1) - \delta(\alpha + s)\Big)
\end{aligned}$$

Again note that $c_-^* - 1 < 0$. Furthermore, note that $\delta(s + \beta c - 1) + \beta\delta(c - 1) - \delta(\alpha + s) \leq 0$ and $-\gamma < 0$. The result then follows.

3. $(trJ_{rev})^2 - 4detJ_{rev} > 0$.

Let the $(i, j)$-entry of $J_{rev}$ be denoted at $a_{ij}$. The following needs to hold

$$(a_{11} + a_{22})^2 - 4a_{11}a_{22} + 4a_{12}a_{21} > 0 \implies (a_{11} - a_{22})^2 + 4a_{12}a_{21} > 0.$$

Note that

$$\begin{aligned} 4a_{12}a_{21} &= 4\beta(\alpha+s)(\delta(c-1)-c+1) \\ &= 4\beta(\alpha+s)(c-1)(\delta-1). \end{aligned}$$

Note also that

$$\begin{aligned} (a_{11}-a_{22})^2 &= \Big(\beta(c-1)-\delta(s+\beta c-1)+(\alpha+\gamma+s)-\beta\delta(c-1)\Big)^2 \\ &= \Big(\beta(c-1)(1-\delta)\Big)^2 + 2\beta(c-1)(1-\delta)(-\delta(s+\beta c-1)+(\alpha+\gamma+s)) \\ &+ \Big(-\delta(s+\beta c-1)+(\alpha+\gamma+s)\Big)^2. \end{aligned}$$

We then have

$$\begin{aligned} (a_{11}-a_{22})^2+4a_{12}a_{21} &= \Big(\beta(c-1)(1-\delta)\Big)^2 + 2\beta(c-1)(1-\delta)(\gamma-\delta(s+\beta c-1)) \\ &- 2\beta(\alpha+s)(c-1)(1-\delta) + \Big(-\delta(s+\beta c-1)+(\alpha+\gamma+s)\Big)^2 \\ &= \Big(\beta(c-1)(1-\delta)-(\alpha+s)\Big)^2 \\ &+ 2\beta(c-1)(1-\delta)(\gamma-\delta(s+\beta c-1)) \\ &+ 2(\alpha+s)(\gamma-\delta(s+\beta c-1)) + \Big(\gamma-\delta(s+\beta c-1)\Big)^2 \\ &= \Big(\beta(c-1)(1-\delta)-(\alpha+s)\Big)^2 \\ &+ 2(\beta(c-1)(1-\delta)+(\alpha+s))(\gamma-\delta(s+\beta c-1)) \\ &+ \Big(\gamma-\delta(s+\beta c-1)\Big)^2 \\ &= \Big(\beta(c-1)(1-\delta)-(\alpha+s)+\gamma-\delta(s+\beta c-1)\Big)^2 \\ &+ 4(\alpha+s)(\gamma-\delta(s+\beta c-1)). \end{aligned}$$

Observe that $\delta(s+\beta c-1) \le 0$ from the conserved quantities (2.7) in the main text. We can conclude that $(a_{11}-a_{22})^2+4a_{12}a_{21} > 0$. □

To summarise, we have that $(s_-^*, c_-^*)$ is a stable node and $0 \le s_-^*, c_-^* < 1$ for $\alpha, \beta, \gamma > 0$ and $\delta \ge 0$. In particular, there is a unique stable node equilibrium at the origin for the case $\delta = 0$.

# 2 Proofs for the stability of the equilibrium in selected reversible MM model reductions

In this section, we sketch proofs of some smaller results claimed in the main paper. Certain steps in these proofs are similar to the steps in the previous section where we showed $(s_-^*, c_-^*)$ is a stable node and $0 \le s_-^*, c_-^* < 1$.

**Lemma 6.** *We have that the following holds*

*1. For Case T.1.i, we have that* $0 < s^* < 1$*,*

*2. For Case T.2a.i, we have that* $0 < c^* < 1$*.*

*Furthermore, these equilibria are attracting.*

*Proof.* We begin with an expression that is positive for the upper bound and the lower bound. Terms are then added, or the expression is manipulated until we obtain the expression for $s^*$ or $c^*$. We provide only a sketch of the proof.

We note that since these are reversible MM cases, then $\delta > 0$.

1. $4(\alpha\tilde{\delta} + 1)(\alpha + \alpha\beta\tilde{\delta} + 1) > 0 \implies s^* = \frac{-\alpha+\alpha\tilde{\delta}-\alpha^2\tilde{\delta}-\alpha\beta\tilde{\delta}+\sqrt{\Delta}}{2(\alpha\tilde{\delta}+1)} < 1$ and $4\alpha^2\tilde{\delta}(\alpha\tilde{\delta} + 1) > 0 \implies s^* > 0$, where $\Delta = \alpha^2\tilde{\delta}^2 + 2\alpha\beta\tilde{\delta}^2 + 2\alpha\tilde{\delta}^2 + 2\alpha\tilde{\delta} + \beta^2\tilde{\delta}^2 - 2\beta\tilde{\delta}^2 + 2\beta\tilde{\delta} + \tilde{\delta}^2 + 2\tilde{\delta} + 1$. The vector field in Table 15 in the main text is a negative quadratic, and so $s^*$ is attracting.

2. $4\beta\tilde{\delta} > 0 \implies c^* = \frac{\tilde{\delta}+\beta\tilde{\delta}+1-\sqrt{\beta^2\tilde{\delta}^2-2\beta\tilde{\delta}^2+2\beta\tilde{\delta}+\tilde{\delta}^2+2\tilde{\delta}+1}}{2\beta\delta} < 1$ and $4\beta\tilde{\delta}^2 > 0 \implies c^* > 0$. The vector field in Table 15 in the main text is a positive quadratic, and so $c^*$ is attracting. □

**Lemma 7.** *We have that the following holds.*

*1. For Case S.3.i, we have that* $s^* = 0$*,*

*2. For Case S.3.ii, we have that* $0 < s^* < 1$*.*

*Furthermore, these equilibria are attracting.*

*Proof.* 1. Observe from Table 13 in the main text that $s^* = 0$ is an equilibrium. Taking the derivative of the vector field and setting $s = 0$, we obtain

$$\frac{1 + \tilde{\delta}(1 - \beta) - \sqrt{\tilde{\delta}^2(\beta - 1)^2 + 1 + 2\beta\tilde{\delta} + 2\tilde{\delta}}}{2\tilde{\delta}}.$$

This is negative and so we have a stable equilibrium.

2. $4(1 + \alpha\tilde{\delta})(1 + \alpha + \alpha\beta\tilde{\delta}) > 0 \implies s^* = \alpha\frac{-(\alpha\tilde{\delta}+1)+\tilde{\delta}(1-\beta)+\sqrt{\Delta}}{2(\alpha\tilde{\delta}+1)} < 1$ and $4\alpha^2\tilde{\delta}(1 + \alpha\tilde{\delta}) > 0 \implies s^* > 0$, where $\Delta = \tilde{\delta}^2(\beta - 1)^2 + (1 + \alpha\tilde{\delta})^2 + 2\tilde{\delta}(\beta + 1)(1 + \alpha\tilde{\delta})$.

There is one other equilibrium $s^*_{other} = \alpha\frac{-(\alpha\tilde{\delta}+\gamma)+\tilde{\delta}(1-\beta)-\sqrt{\Delta}}{2(\alpha\tilde{\delta}+1)} < 0$. At $s = 0, 1$, the vector field (see Table 13 in the main text) is as follows

$$s = 0 \implies \alpha\frac{\tilde{\delta}(\beta + 1) + 1 - \sqrt{\tilde{\delta}^2(\beta - 1)^2 + 1 + 2\beta\tilde{\delta} + 2\tilde{\delta}}}{2\tilde{\delta}}, \quad s = 1 \implies -\beta$$

It remains to check if the value of the vector field at $s = 0$ is positive. One can check that $4\beta\tilde{\delta}^2 > 0$ implies this is the case.

Hence, since the vector field is positive at $s = 0$, negative at $s = 1$, we can conclude that the equilibrium $0 < s^* < 1$ is attracting. □
